# Supplementary material for: The Case for Translation-Invariant Self-Attention in Transformer-Based Language Models
Source: arXiv:2106.01950 source file (2021-06-03)
Supplement: Supplementary file 1 [file multifix_suppl1.tex]

\begin{figure*}[h!]
	\centering
	\hfill
	\begin{subfigure}[t]{0.485\textwidth}
		\centering
		\includegraphics[width=\textwidth]{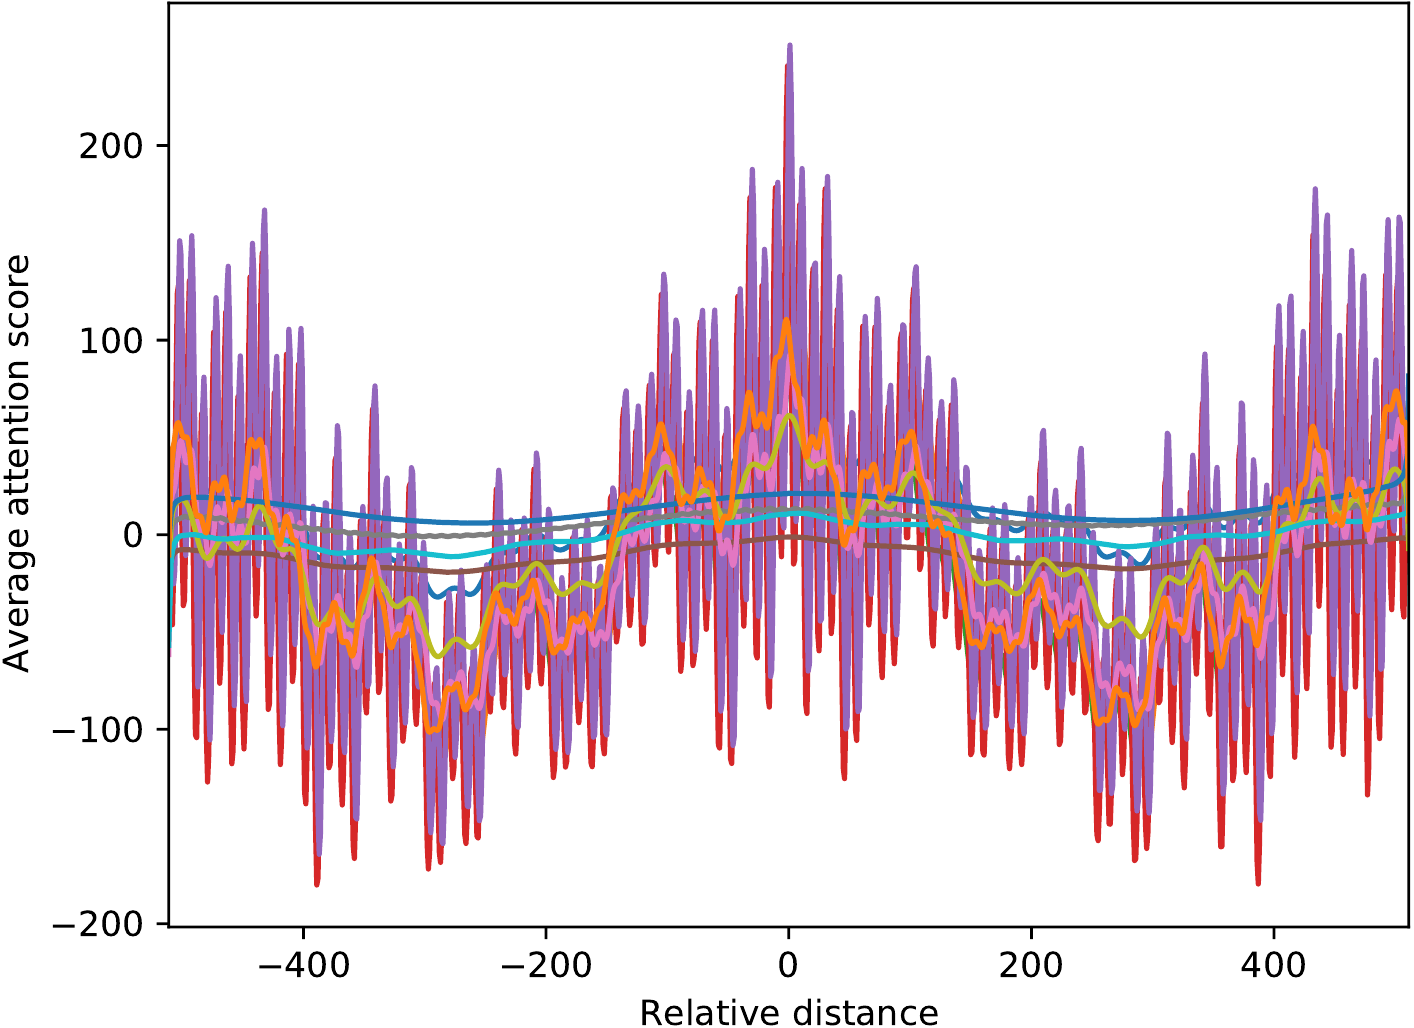}
		%\caption{$S=1$}
		%\label{sfig:s1}
	\end{subfigure}
	\hfill
	\hfill
	\begin{subfigure}[t]{0.485\textwidth}
		\centering
		\includegraphics[width=\textwidth]{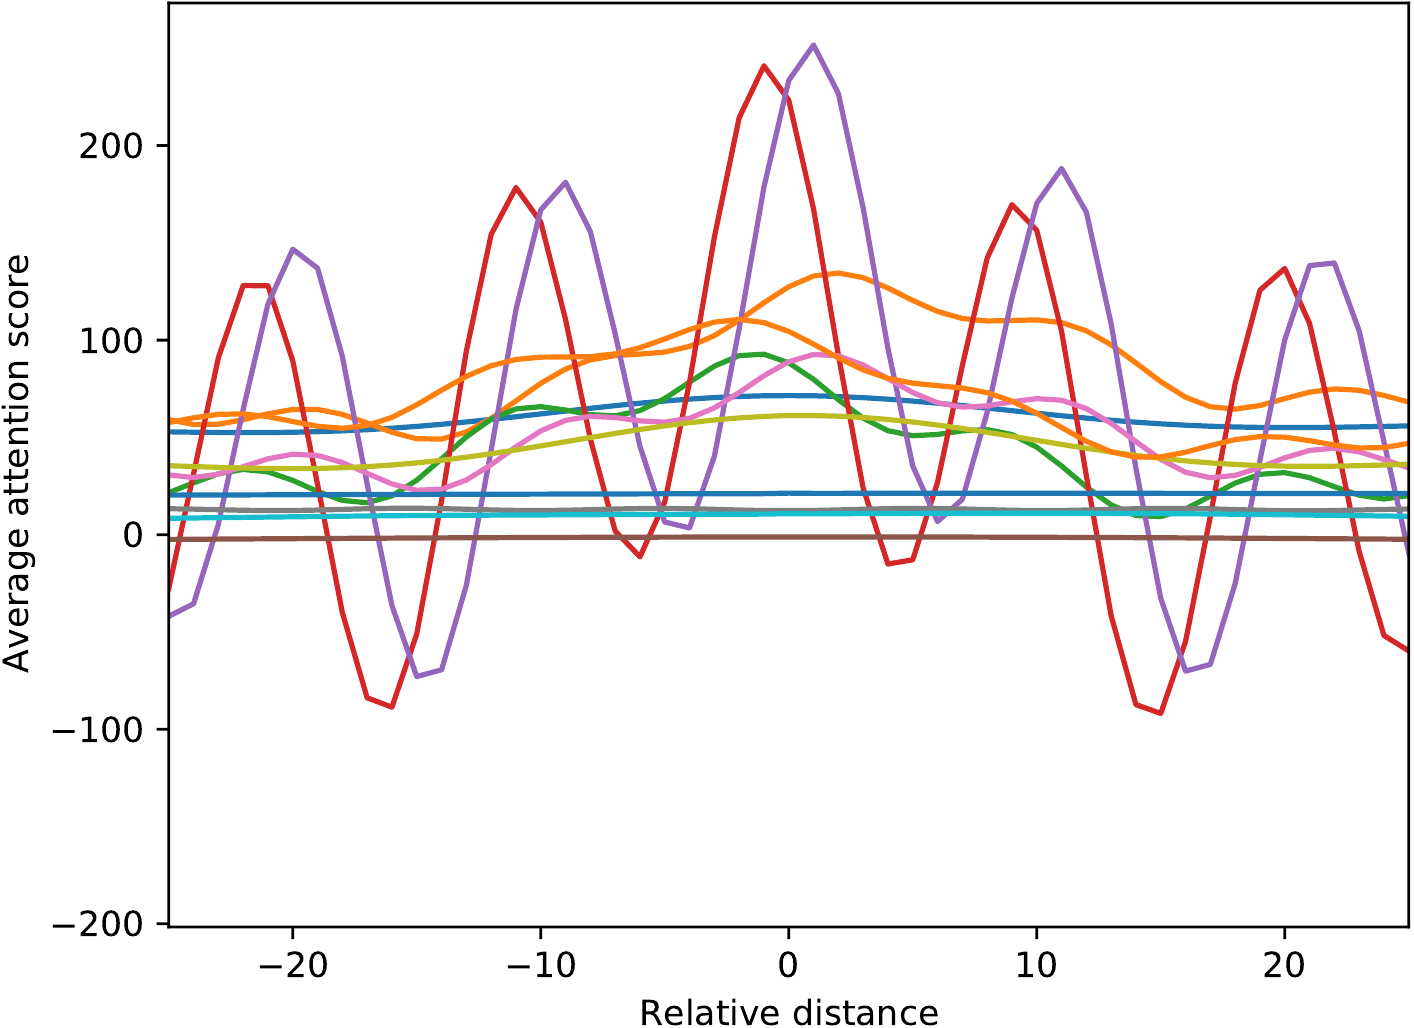}
		%\caption{$S=5$}
		%\label{sfig:s5}
	\end{subfigure}
	\hfill
	\caption{Plot over the average positional embedding contribution to the attention scores in the attention module for different relative position distances. The plots show that the learned position embeddings in the ALBERT model give rise to sinusoidal contributions to the attention scores, both on macro and micro scales.}
	\label{fig:albert_pos_attention_scores}
    \vspace{-1em}
\end{figure*}
